# Supplementary material for: Vibronic State-Specific Modelling of High-Speed Nitrogen Shocked Flows. Part II: Shock Tube Simulations
Source: arXiv:2308.05164 source file (2023-08-09)
Supplement: Supplementary file 1 [file Appendix_B.tex]

\section{The database of kinetic processes}
\label{chapter:Database_kinetic}
\Cref{tab:kin_h_synopsis,tab:kin_e_synopsis,tab:rad_mol_synopsis,tab:rad_ato_synopsis} present the kinetic processes database developed in this work. In the case of \Cref{tab:kin_h_synopsis,tab:kin_e_synopsis} which are with respect to the regarded collisional processes, a codename for the type of process was defined to simplify the description of the process. It consists of three terms separated by hyphens. If the process corresponds solely to a transition in the internal energy modes of the collision partners, the first term of the codename will correspond to a set of capital letters each one representing the involved internal energy modes (``V'' from ``vibrational'' or/and ``E'' from ``electronic''). If the process corresponds to a bond breaking or/and forming of the internal structure, the first term will be defined by a set of capital letters, each one representing a type of bond breaking or forming (``I'' from ``ionisation'', ``R'' from ``recombination'', ``D'' from ``dissociation'' or ``A'' from ``association''). The second and third terms correspond to labels of minuscule letters representing the type of the collision partners (``h'' from ``heavy species'', ``m'' from ``molecular particle'', ``a'' from ``atomic particle'', or ``e'' from ``electron'').

\begingroup
\centerline{\begin{threeparttable}
\setlength\tabcolsep{4pt} %Change width of the columns (default value is 6pt)
 % General space between rows (1 standard)
\centering
\caption{Collisional processes due to heavy particle impact for which forward rate constants were obtained. The symbol after the reference in the column ``Reference'' represents the physical quantity which was extracted from it: process cross section (if $\sigma_p$), average process cross section (if $\sigma_{p,\text{av}}$) or forward rate constant (if $k_f$).}
\begin{scriptsize}
\begin{tabular}{cccc}
\toprule
Type & Chemical equation & Remarks & Reference \\
\midrule
V-m-h & $\ch{N_2}\left(e,v\right)\ch{ + M}\ch{ <=> N2}\left(e,v'\right)\ch{ + M}$ & \parbox{7cm}{\centering \text{ }\\ $e\in\{\text{X},\text{A},\text{B},\text{W},\text{B}',\text{a}',\text{a},\text{w},\text{A}',\text{C},\text{b},\text{c}_3,\text{c}'_4,\text{b}',\text{o}_3\}$, \\ $\forall\,v$, $\forall\,v'>v$ and $\ch{M} \in \{\ch{N2}, \ch{N2+}, \ch{N}, \ch{N+}\}$\\ \text{ }} & This work (\tnote{a} )\\
\greymidrule
V-m-h & $\ch{N_2+}\left(e,v\right)\ch{ + M}\ch{ <=> N2+}\left(e,v'\right)\ch{ + M}$ & \parbox{7cm}{\centering \text{ }\\ $e\in\{\text{X},\text{A},\text{B},\text{D},\text{C}\}$, $\forall\,v$, $\forall\,v'>v$\\ and $\ch{M} \in \{\ch{N2}, \ch{N2+}, \ch{N}, \ch{N+}\}$\\ \text{ }} & This work (\tnote{a} )\\
\midrule
VE-m-a & $\ch{N2}\left(\text{A},v\right)\ch{ + N}({}^4\text{S}_\text{u})\ch{ <=> N2}\left(\text{X},v'\right)\ch{ + N}({}^2\text{P}_\text{u})$ & $\forall\,v,$ and $\forall\,v'$ & \cite{piper1989}-$k_f$\\
\greymidrule
VE-m-a & $\ch{N2}\left(\text{A},v\right)\ch{ + N}({}^4\text{S}_\text{u})\ch{ <=> N2}\left(\text{B},v'\right)\ch{ + N}({}^4\text{S}_\text{u})$ & $\forall\,v,$ and $\forall\,v'$ & \cite{bachmann1993}-$\sigma_{p,\text{av}}$\\
\greymidrule
VE-m-a & $\ch{N2}\left(\text{W},v\right)\ch{ + N}({}^4\text{S}_\text{u})\ch{ <=> N2}\left(\text{B},v'\right)\ch{ + N}({}^4\text{S}_\text{u})$ & $\forall\,v,$ and $\forall\,v'$ & \cite{bachmann1993}-$\sigma_{p,\text{av}}$\\
\greymidrule
VE-m-a & $\ch{N2}\left(\text{A}',0\right)\ch{ + N}({}^4\text{S}_\text{u})\ch{ <=> N2}\left(\text{B},10\right)\ch{ + N}({}^4\text{S}_\text{u})$ & --- & \cite{ottinger1994a}-$\sigma_{p,\text{av}}$\\
\greymidrule
VE-m-m & $\ch{N2}\left(\text{A},v_1\right)\ch{ + N2}\left(\text{X},v_2\right)\ch{ <=> N2}\left(\text{X},v'_1\right)\ch{ + N2}\left(\text{X},v'_2\right)$ & $\forall\,v_1$, $\forall\,v_2$, $\forall\,v'_1$ and $\forall\,\,v_2'$ & \cite{levron1978}-$k_f$\\
\greymidrule
VE-m-m & $\ch{N2}\left(\text{A},v_1\right)\ch{ + N2}\left(\text{X},v_2\right)\ch{ <=> N2}\left(\text{B},v'_1\right)\ch{ + N2}\left(\text{X},v'_2\right)$ & $\forall\,v_1$, $\forall\,v_2$, $\forall\,v'_1$ and $\forall\,\,v_2'$ & \cite{bachmann1993}-$\sigma_{p,\text{av}}$\\
\greymidrule
VE-m-m & $\ch{N2}\left(\text{A},v_1\right)\ch{ + N2}\left(\text{A},v_2\right)\ch{ <=> N2}\left(\text{B},v'_1\right)\ch{ + N2}\left(\text{X},v'_2\right)$ & $\forall\,v_1$, $\forall\,v_2$, $\forall\,v'_1$ and $\forall\,\,v_2'$ & \cite{piper1988b}-$k_f$\\
\greymidrule
VE-m-m & $\ch{N2}\left(\text{A},v_1\right)\ch{ + N2}\left(\text{A},v_2\right)\ch{ <=> N2}\left(\text{C},v'_1\right)\ch{ + N2}\left(\text{X},v'_2\right)$ & $\forall\,v_1$, $\forall\,v_2$, $\forall\,v'_1$ and $\forall\,\,v_2'$ & \cite{piper1988a}-$k_f$\\
\greymidrule
VE-m-m & $\ch{N2}\left(\text{W},v_1\right)\ch{ + N2}\left(\text{X},v_2\right)\ch{ <=> N2}\left(\text{B},v'_1\right)\ch{ + N2}\left(\text{X},v'_2\right)$ & $\forall\,v_1$, $\forall\,v_2$, $\forall\,v'_1$ and $\forall\,\,v_2'$ & \cite{bachmann1993}-$\sigma_{p,\text{av}}$\\
\greymidrule
VE-m-m & $\ch{N2}\left(\text{A}',0\right)\ch{ + N2}\left(\text{X},0\right)\ch{ <=> N2}\left(\text{B},10\right)\ch{ + N2}\left(\text{X},0\right)$ & --- & \cite{ottinger1994a}-$\sigma_{p,\text{av}}$\\
\midrule
E-a-h & $\ch{N}\left(e\right)\ch{ + M <=> N}\left(e'\right)\ch{ + M}$ & $\forall e$, $\forall e'>e$ and $\text{M}\in\{\ch{N},\ch{N2}\}$ & \cite{annaloro2014b}-$k_f$ \\
\greymidrule
E-a-h & $\ch{N+}\left(e\right)\ch{ + M <=> N+}\left(e'\right)\ch{ + M}$ & $\forall e$, $\forall e'>e$ and $\text{M}\in\{\ch{N},\ch{N2}\}$ & \cite{annaloro2014b}-$k_f$ \\
\midrule
D-m-h & $\ch{N2}\left(e,v\right)\ch{ + M}\ch{ <=> N}\left(e'_1\right)\ch{ + N}\left(e'_2\right)\ch{ + M}$ & \parbox{7cm}{\centering \text{ }\\$e\in\{\text{X},\text{A},\text{B},\text{W},\text{B}',\text{a}',\text{a},\text{w},\text{A}',\text{C},\text{b},\text{b}'\}$,\\ $\forall\,v$ and  $\ch{M} \in \{\ch{N2}, \ch{N2+}, \ch{N}, \ch{N+}\}$\\ \text{ }} & This work (\tnote{a} )\\
\greymidrule
D-m-h & $\ch{N2+}\left(e,v\right)\ch{ + M}\ch{ <=> N}\left(e'_1\right)\ch{ + N+}\left(e'_2\right)\ch{ + M}$ & \parbox{7cm}{\centering \text{ }\\$e\in\{\text{X},\text{A},\text{B},\text{D},\text{C}\}$,\\ $\forall\,v$ and  $\ch{M} \in \{\ch{N2}, \ch{N2+}, \ch{N}, \ch{N+}\}$\\ \text{ }} & This work (\tnote{a} )\\
\midrule
I-a-h & $\ch{N}\left(e\right)\ch{ + M <=> N+}\left({}^3\text{P}\right)\ch{ + M + e-}$ & $\forall e$ and $\text{M}\in\{\ch{N},\ch{N2}\}$ & \cite{annaloro2014b}-$k_f$ \\
\midrule
IR-m-a & $\ch{N2}\left(\text{X},v\right)\ch{ + N+}({}^3\text{P})\ch{ <=> N2+}\left(\text{X},v'\right)\ch{ + N}({}^4\text{S}_{\text{u}})$ & VRP on $v$ and $v'$ from case $v=0$ and $\sum_{v'}$ & \cite{freysinger1994}-$\sigma_p$ \\
\bottomrule
\end{tabular}
\label{tab:kin_h_synopsis}
\end{scriptsize}
\begin{scriptsize}
\begin{tablenotes}
\item[a]{Note that although the respective chemical equation doesn't show any possible transition in the vibrational level (or even dissociation) of the second collision partner (if it is a molecular particle), such possibility is implicit.
}\\
\end{tablenotes}
\end{scriptsize}
\end{threeparttable}}
\endgroup
\begingroup
\centerline{\begin{threeparttable}
\setlength\tabcolsep{0pt} %Change width of the columns (default value is 6pt)
 % General space between rows (1 standard)
\centering
\caption{Collisional processes due to electron impact for which forward rate constants were obtained. The symbol after the reference in the column ``Reference'' represents the physical quantity which was extracted from it: process cross section (if $\sigma_p$), average process cross section (if $\sigma_{p,\text{av}}$) or forward rate constant (if $k_f$).}
\begin{scriptsize}
\begin{tabular}{cccc}
\toprule
Type & Chemical equation & Remarks & Reference \\
\midrule
V-m-e & $\ch{N_2}\left(\text{X}{}^1\Sigma_{\text{g}}^+,\,v\right)\ch{ + e- <=> N_2}\left(\text{X}{}^1\Sigma_{\text{g}}^+,\,v'\right)\ch{ + e-}$ & $\forall v$ and $\forall\,v'>v$, ADV & \cite{laporta2014}-$\sigma_p$ (from \cite{Phys4Entry})\\
\midrule
\multirow{4}{*}{\parbox{1.2cm}{\centering \text{ }\\ \text{ }\\ \text{ }\\ \text{ }\\VE-m-e}} & \multirow{4}{*}{\parbox{5cm}{\centering \text{ }\\ \text{ }\\ \text{ }\\ \text{ }\\$\ch{N2}\left(\text{X},v\right)\ch{ + e-}\ch{ <=> N2}\left(e',v'\right)\ch{ + e-}$}}  & \parbox{7cm}{\centering \text{ }\\$e'\in\{\text{A},\text{B},\text{W},\text{B}',\text{a}',\text{a},\text{w},\text{C}\}$,\\VRP on $v$ and $v'$ from case $v=0$ and $\sum_{v'}$\\ \text{ }} & \cite{brunger2003}-$\sigma_p$\\
 & & \parbox{9cm}{\centering \text{ } \\$e'\in\{\text{c}_3,\text{o}_3\}$, VRP on $v$ and $v'$ from case $v=0$ and $\sum_{v'}$ \\ \text{ }} & \cite{malone2012}-$\sigma_p$\\
 & & \parbox{9cm}{\centering \text{ } \\$e'\in\{\text{b},\text{c}'_4,\text{b}'\}$, VRP on $v$ and $v'$ from case $v=0$ and $\sum_{v'}$\\ \text{ }} & \cite{itikawa2006}-$\sigma_p$\\
 & & \parbox{9cm}{\centering \text{ }\\$e'=\text{A}'$, Assumption of same reference values as for $e'=\text{A}$,\\VRP on $v$ and $v'$ from case $v=0$ and $\sum_{v'}$\\ \text{ }} & ---\\
\greymidrule
\multirow{2}{*}{\parbox{1.2cm}{\centering \text{ }\\ \text{ }\\ \text{ }\\VE-m-e}} & \multirow{2}{*}{\parbox{5cm}{\centering \text{ }\\ \text{ }\\ \text{ }\\$\ch{N2+}\left(\text{X},v\right)\ch{ + e-}\ch{ <=> N2+}\left(e',v'\right)\ch{ + e-}$}} & \parbox{9cm}{\centering \text{ }\\$e'=\text{B}$, $v=0$ and $v'=0$,\\Remainder of $v$ and $v'$: VRP from case $v=0$ and $v'=0$\\ \text{ }}  & \cite{crandall1974}-$\sigma_p$\\
 & & \parbox{9cm}{\centering \text{ }\\$e'\in\{\text{A},\text{D},\text{C}\}$,\\ Assumption of same reference values as for $e'=\text{B}$, $v=0$ and $v'=0$,\\Remainder of $v$ and $v'$: VRP from case $v=0$ and $v'=0$\\ \text{ }}  & ---\\
\midrule
\multirow{2}{*}{E-a-e} & \multirow{2}{*}{$\ch{N}\left(e\right)\ch{ + e- <=> N}\left(e'\right)\ch{ + e-}$ } & $(e,e')\in\{({}^4\text{S}_\text{u},{}^2\text{D}_\text{u}),({}^4\text{S}_\text{u},{}^2\text{P}_\text{u}),({}^2\text{D}_\text{u},{}^2\text{P}_\text{u})\}$ & \cite{berrington1975}-$\sigma_p$\\
 & &  Remainder of $(e,e')$, with $e'>e$ & \cite{panesi2009}-$k_f$ \\
\greymidrule
E-a-e & $\ch{N+}\left(e\right)\ch{ + e- <=> N+}\left(e'\right)\ch{ + e-}$ & $\forall e$ and $\forall e'>e$ & \cite{panesi2009}-$k_f$ \\
\midrule
\multirow{2}{*}{D-m-e} & \multirow{2}{*}{$\ch{N_2}\left(\text{X}{}^1\Sigma_{\text{g}}^+,\,v\right)\ch{ + e- <=> N}\left(e_1'\right)\ch{ + N}\left(e_2'\right)\ch{ + e-}$} & $\forall\,v$, $(e_1',e_2')=({}^4\text{S}_\text{u},{}^4\text{S}_\text{u})$, ADV & \cite{laporta2014}-$\sigma_p$ (from \cite{Phys4Entry}) \\
& & $\forall\,v$, $(e_1',e_2')=({}^4\text{S}_\text{u},{}^2\text{D}_\text{u})$, ADV & \cite{capitelli1998}-$\sigma_p$ (from \cite{Phys4Entry}) \\
\midrule
\multirow{3}{*}{\parbox{1.2cm}{\centering \text{ }\\ \text{ }\\ \text{ }\\ DR-m-e}} & \multirow{2}{*}{\parbox{5cm}{\centering \text{ }\\ \text{ }\\ \text{ }\\ $\ch{N2+}\left(\text{X}{}^2\Sigma_{\text{g}}^+,\,v\right)\ch{ + e^- <=> N}\left(e_1'\right)\ch{ + N}\left(e_2'\right)$}} & \parbox{9cm}{\centering  $v\in\{0,2\}$ and $(e'_1,e'_2)\in\{({}^4\text{S}_\text{u},{}^2\text{D}_\text{u}),({}^4\text{S}_\text{u},{}^2\text{P}_\text{u}),({}^2\text{D}_\text{u},{}^2\text{D}_\text{u})\}$,\\ \text{ }} & \multirow{2}{*}{\parbox{1cm}{\centering \text{ }\\ \text{ }\\ \text{ }\\ \cite{guberman2014}-$k_f$}} \\
 & & \parbox{9cm}{\centering $v\in\{1,3,4\}$ and \\ $(e'_1,e'_2)\in\{({}^4\text{S}_\text{u},{}^2\text{D}_\text{u}),({}^4\text{S}_\text{u},{}^2\text{P}_\text{u}),({}^2\text{D}_\text{u},{}^2\text{D}_\text{u}),({}^2\text{D}_\text{u},{}^2\text{P}_\text{u})\}$,\\ \text{ }} & \\
 & & \parbox{9cm}{\centering Remainder of $v$ with\\ $(e'_1,e'_2)\in\{({}^4\text{S}_\text{u},{}^2\text{D}_\text{u}),({}^4\text{S}_\text{u},{}^2\text{P}_\text{u}),({}^2\text{D}_\text{u},{}^2\text{D}_\text{u}),({}^2\text{D}_\text{u},{}^2\text{P}_\text{u})\}$:\\ VRP from case $v=4$} & \\
\midrule
I-m-e & $\ch{N_2}\left(\text{X}{}^1\Sigma_{\text{g}}^+,\,v\right)\ch{ + e^- <=> N_2^+}\left(e',v'\right)\ch{ + 2 e^-}$ & \parbox{9cm}{\centering $\forall\,v$ and $e'\in\{\text{X},\text{A},\text{B}\}$, ADV, VRP on $v'$ from case $\sum_{v'}$} & \cite{laricchiuta2006}-$\sigma_p$ (from \cite{Phys4Entry})\\ 
\greymidrule
\multirow{3}{*}{I-a-e} & \multirow{3}{*}{$\ch{N}\left(e\right)\ch{ + e- <=> N+}\left({}^3\text{P}\right)\ch{ + 2 e-}$} & $e={}^4\text{S}_\text{u}$ & \cite{brook1978}-$\sigma_p$\\
 & & $e\in\{{}^2\text{D}_\text{u},{}^2\text{P}_\text{u}\}$ & \cite{wang2014}-$\sigma_p$ \\
 & & Remainder of $e$ & \cite{panesi2009}-$k_f$ \\
\bottomrule
\end{tabular}
\label{tab:kin_e_synopsis}
\end{scriptsize}
\end{threeparttable}}
\endgroup

\begingroup
\centerline{\begin{threeparttable}
\setlength\tabcolsep{20pt} %Change width of the columns (default value is 6pt)
 % General space between rows (1 standard)
\centering
\caption{Molecular spontaneous emission processes for which Einstein coefficients were obtained. The symbol after the reference in the column ``Reference'' represents the quantity which was extracted from it: Einstein coefficient (if $A$) or sum of the electronic-vibrational transition moments  (if $\sum R_e^2$).}
\begin{scriptsize}
\begin{tabular}{ccccc}
\toprule
Species & Electronic system & $e$ - $e'$ & $(v_\text{max},v'_\text{max})$ & Reference \\
\midrule
\multirow{10}{*}{\ch{N2}} & Vegard-Kaplan &  A${}^3\Sigma_\text{u}^+$ - X${}^1\Sigma_\text{g}^+$ & $(21,21)$ & \cite{quin2017} - $A$ (from \cite{quin2017data})\\ 
 & First positive & B${}^3\Pi_\text{g}$ - A${}^3\Sigma_\text{u}^+$ & $(21,21)$ & \cite{laux1992} - $A$\\
 & Wu-Benesch & W${}^3\Delta_\text{u}$ - B${}^3\Pi_\text{g}$ & $(21,17)$ & \cite{quin2017} - $A$ (from \cite{quin2017data})\\
 & IR afterglow & B$'{}^3\Sigma_\text{u}^-$ - B${}^3\Pi_\text{g}$ & $(21,21)$ & \cite{quin2017} - $A$ (from \cite{quin2017data})\\
 & Lyman-Birge-Hopfield & a${}^1\Pi_\text{g}$ - X${}^1\Sigma_\text{g}^+$ & $(21,21)$ & \cite{quin2017} - $A$ (from \cite{quin2017data})\\
 & Second positive & C${}^3\Pi_\text{u}$ - B${}^3\Pi_\text{g}$ & $(4,21)$ & \cite{laux1992} - $A$\\ 
 & Birge-Hopfield I &  b${}^1\Pi_\text{u}$ - X${}^1\Sigma_\text{g}^+$ & $(24,60)$ & \cite{liebhart2010} - $\sum R_e^2$\\
 & Worley-Jenkins &  c$_3{}^1\Pi_\text{u}$ - X${}^1\Sigma_\text{g}^+$ & $(11,60)$ & \cite{liebhart2010} - $\sum R_e^2$\\ 
 & Carroll-Yoshino &  c$_4'{}^1\Sigma_\text{g}^+$ - X${}^1\Sigma_\text{g}^+$ & $(11,60)$ & \cite{liebhart2010} - $\sum R_e^2$\\
 & Birge-Hopfield II &  b$'{}^1\Sigma_\text{u}^+$ - X${}^1\Sigma_\text{g}^+$ & $(46,60)$ & \cite{liebhart2010} - $\sum R_e^2$\\
 & Worley &  o$_3{}^1\Pi_\text{u}$ - X${}^1\Sigma_\text{g}^+$ & $(21,60)$ & \cite{liebhart2010} - $\sum R_e^2$\\
\hline
\multirow{3}{*}{\ch{N2+}} & Meinel & A${}^2\Pi_\text{u}$ - X${}^2\Sigma_\text{g}^+$ & $(27,27)$ & \cite{quin2017} - $A$ (from \cite{quin2017data})\\
 & First negative &  B${}^2\Sigma_\text{u}^+$ - X${}^2\Sigma_\text{g}^+$ & $(12,21)$ & \cite{laux1992} - $A$\\
 & Second negative & C${}^2\Sigma_\text{u}^+$ - X${}^2\Sigma_\text{g}^+$ & $(6,27)$ & \cite{quin2017} - $A$ (from \cite{quin2017data})\\
\bottomrule
\end{tabular}
\label{tab:rad_mol_synopsis}
\begin{tablenotes}
%\item[a]{The data were directly sent by Heiko Liebhart to the IPFN group.}\\
\end{tablenotes}
\end{scriptsize}
\end{threeparttable}}
\endgroup
\vspace{17.5pt}

\begingroup
\centerline{\begin{threeparttable}
\setlength\tabcolsep{52.5pt} %Change width of the columns (default value is 6pt)
 % General space between rows (1 standard)
\centering
\caption{Atomic spontaneous emission processes for which Einstein coefficients were computed.}
\begin{scriptsize}
\begin{tabular}{ccc}
\toprule
Species & Number of processes & Reference \\
\midrule
\ch{N} & 279 (\tnote{a} ) & NIST\cite{NIST}\\
\ch{N+} & 276 (\tnote{a} ) & NIST\cite{NIST}\\
\bottomrule
\end{tabular}
\label{tab:rad_ato_synopsis}
\begin{tablenotes}
\item[a]{As a reminder to the reader: representative Einstein coefficients were computed considering the lumping procedure performed on the split electronic levels.}\\
\end{tablenotes}
\end{scriptsize}
\end{threeparttable}}
\endgroup
